# Supplementary material for: HumanScore: Benchmarking Human Motions in Generated Videos
Source: arXiv:2604.20157 source file (2026-11-03)
Supplement: Supplementary file 3 [file b_usage.tex]

\section{Availability and Broader Usage}

We collected a set of 102 prompts spanning diverse motion types and difficulty levels to comprehensively evaluate video generators. For an apples-to-apples comparison, we evaluate all models using the same prompt set, thereby restricting the benchmark to controlled settings.

Our proposed metrics are \emph{not} limited to these predefined prompts. They are designed to be motion-agnostic and can be applied directly to in-the-wild videos; accordingly, our evaluation pipeline takes RGB monocular video as input and does not require curated prompts. Although the benchmark focuses on single-person videos, the metrics extend naturally to multi-person settings with standard preprocessing (e.g., per-person tracking and segmentation), after which the same evaluation can be applied to each person separately.
